# Supplementary material for: Non-perturbative calculation of orbital- and spin effects in molecules subject to non-uniform magnetic fields
Source: arXiv:1803.04776 source file (2018-03-13)
Supplement: Supplementary file 1 [file supp_info.pdf]

**Non-perturbative calculation of orbital- and spin effects in molecules subject to non-uniform magnetic fields**

Sangita Sen<sup>1, a)</sup> and Erik I. Tellgren<sup>1, b)</sup>

*Hylleraas Centre for Quantum Molecular Sciences, Department of Chemistry,  
University of Oslo, P.O. Box 1033 Blindern, N-0315 Oslo,  
Norway*

---

<sup>a)</sup>Electronic mail: sangita.sen@kjemi.uio.no

<sup>b)</sup>Electronic mail: erik.tellgren@kjemi.uio.no

## I. GEOMETRIES

For the list of molecules studied by us, the Cartesian co-ordinates in atomic units are listed below.

### CHFC12

|    |           |           |           |
|----|-----------|-----------|-----------|
| C  | 0.000000  | 0.000000  | 0.000000  |
| F  | 0.000000  | 2.402282  | -0.856309 |
| Cl | 2.780473  | -1.558378 | -1.056699 |
| Cl | -2.780473 | -1.558378 | -1.056699 |
| H  | 0.000000  | 0.000000  | 2.050822  |

### CHFC1Br

|    |           |           |           |
|----|-----------|-----------|-----------|
| C  | 0.000000  | 0.000000  | 0.000000  |
| F  | 0.000000  | 2.395362  | -0.866228 |
| Cl | 2.739277  | -1.588887 | -1.077879 |
| Br | -3.106400 | -1.686152 | -1.088828 |
| H  | 0.000000  | 0.000000  | 2.049631  |

### CHBr2

|    |           |           |           |
|----|-----------|-----------|-----------|
| C  | 0.000000  | 0.000000  | 0.000000  |
| F  | 0.000000  | 2.389551  | -0.874127 |
| Br | 3.063900  | -1.717548 | -1.111584 |
| Br | -3.063900 | -1.717548 | -1.111584 |
| H  | 0.000000  | 0.000000  | 2.048722  |

### H2O2, dihedral = 120 deg

|   |          |           |           |
|---|----------|-----------|-----------|
| H | 0.902593 | -1.563337 | -1.726149 |
| H | 0.902593 | 1.563337  | 1.726149  |
| O | 0.000000 | 0.000000  | -1.407846 |
| O | 0.000000 | 0.000000  | 1.407846  |

### H2

|   |          |          |          |
|---|----------|----------|----------|
| H | 0.000000 | 0.000000 | 0.000000 |
| H | 0.000000 | 0.000000 | 0.740000 |

### O2

|   |          |          |          |
|---|----------|----------|----------|
| O | 0.000000 | 0.000000 | 0.000000 |
| O | 0.000000 | 0.000000 | 2.287000 |
